# Supplementary material for: UniT: Unified Multimodal Chain-of-Thought Test-time Scaling
Source: arXiv:2602.12279 source file (2026-06-12)
Supplement: Supplementary file 1 [file supp.tex]

\begin{figure*}[]
    \centering
    \includegraphics[width=0.99\linewidth]{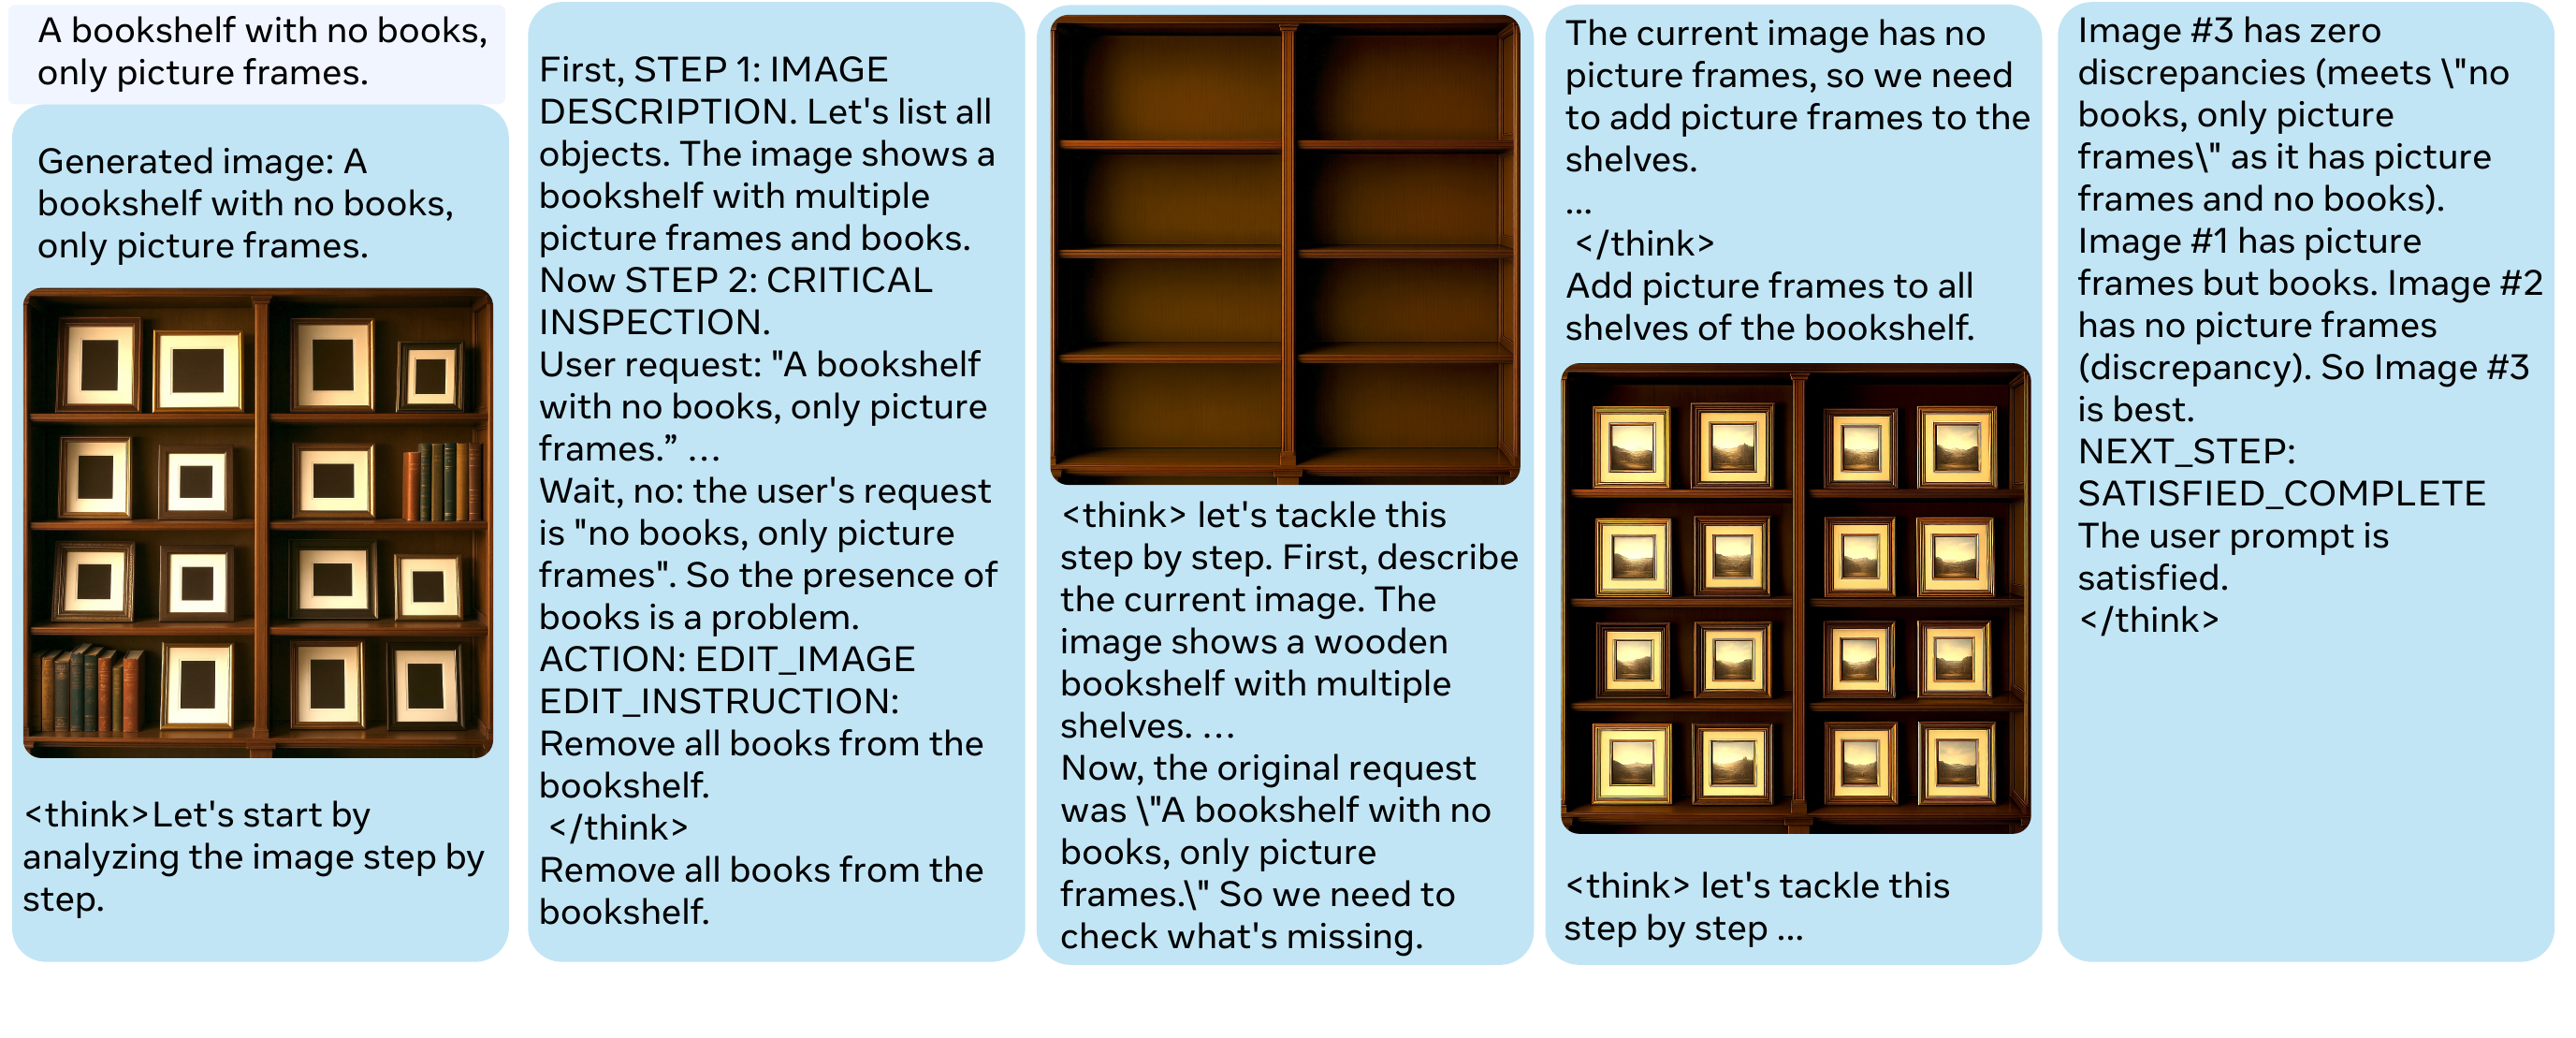}
    \vspace{-5mm}
    \caption{\textbf{Example of agentic chain-of-thought training data demonstrating cognitive behaviors.} The model progressively refines a bookshelf image through explicit reasoning (\texttt{<think>} blocks), demonstrating verification (checking against ``no books, only picture frames''), subgoal decomposition (sequential steps to fix issues), and content memory (comparing Image \#1, \#2, \#3). This multi-turn trajectory teaches the model to identify errors, plan corrections, and determine task completion through test-time computation.}
    \label{fig:verification}
\end{figure*}
